# Supplementary material for: Controllable Hand Grasp Generation for HOI and Efficient Evaluation Methods
Source: arXiv:2501.15839 source file (2025-01-27)
Supplement: Supplementary file 1 [file appendix.tex]

\appendix

\section{APPENDIX}

\section{Pseudocode for Computing Evaluation Metric $f$-FID}

We provide the Pseudocode for computing the \( f \)-FID score. Algorithm~\ref{algo:mean_cov}, calculates the mean vector and covariance matrix of a given population after transforming each hand pose using the Hand Orientation Representation (HOR) function \( f \). Building on this, Algorithm~\ref{algo:ffid}, leverages the computed means and covariances from two distinct populations to determine their similarity.

\begin{algorithm}[H]
	\caption{Compute Mean and Covariance for a Population}
	\label{algo:mean_cov}
	\begin{algorithmic}[1]
		\REQUIRE A population of hand poses $P$, and a descriptor function $f$
		\ENSURE The mean vector $\boldsymbol{\mu}^f$ and covariance matrix $\boldsymbol{\Sigma}^f$
		
		\STATE Initialize $\boldsymbol{\mu}^f = \mathbf{0}$ and $\boldsymbol{\Sigma}^f = \mathbf{0}$
		\FOR {each $\mathbf{p} \in P$}
			\STATE Transform the hand pose using HOR: $\mathbf{q} = f(\mathbf{p})$
			\STATE Update the mean: $\boldsymbol{\mu}^f \mathrel{+}= \mathbf{q}$
			\STATE Update  covar. $\boldsymbol{\Sigma}^f \mathrel{+}= \left(\mathbf{q} - \boldsymbol{\mu}^f\right) \left(\mathbf{q} - \boldsymbol{\mu}^f\right)^\top$
		\ENDFOR
		\STATE Normalize the mean: $\boldsymbol{\mu}^f \mathrel{/}= |P|$
		\STATE Normalize the covariance: $\boldsymbol{\Sigma}^f \mathrel{/}= |P|$
		
		\STATE \textbf{Return} $\boldsymbol{\mu}^f$, $\boldsymbol{\Sigma}^f$
	\end{algorithmic}
\end{algorithm}

\begin{algorithm}[t]
	\caption{Calculating $f$-FID Score for Hand Pose Models}
	\label{algo:ffid}
	\begin{algorithmic}[1]
		\REQUIRE Two populations of hand poses $P_1$, $P_2$, and a descriptor function $f$
		\ENSURE The $f$-FID score
		
		\STATE Call \textbf{Algorithm \ref{algo:mean_cov}} with $P_1$ to obtain $\boldsymbol{\mu}_1^f$ and $\boldsymbol{\Sigma}_1^f$
		
		\STATE Call \textbf{Algorithm \ref{algo:mean_cov}} with $P_2$ to obtain $\boldsymbol{\mu}_2^f$ and $\boldsymbol{\Sigma}_2^f$

		\STATE Calculate the difference of means $\boldsymbol{\mu}_{\text{diff}}$:
		\[
		\boldsymbol{\mu}_{\text{diff}} = \|\boldsymbol{\mu}_1^f - \boldsymbol{\mu}_2^f\|^2
		\]
		\STATE Calculate the trace of the covariance matrices:
		\[
		\text{tr}_{\Sigma} = \text{Tr}(\boldsymbol{\Sigma}_1^f + \boldsymbol{\Sigma}_2^f - 2 \sqrt{\boldsymbol{\Sigma}_1^f \boldsymbol{\Sigma}_2^f})
		\]
		\STATE Compute the $f$-FID score:
		\[
		f\text{-FID} = \boldsymbol{\mu}_{\text{diff}} + \text{tr}_{\Sigma}
		\]
		
		\STATE \textbf{Step 4: Return the $f$-FID score}
	\end{algorithmic}
\end{algorithm}

\section{Implementation Details of the Hand Pose Generation Model}

We utilize two types of encoders: a UNet encoder and a VAE encoder. The model with the UNet encoder is trained end-to-end, whereas the model with the VAE encoder is kept frozen during training. Tables \ref{table:unetEnc} and \ref{table:vaeEnc} provide detailed descriptions of the UNet and VAE encoders, respectively. The rows in each table are listed in the order that the layers appear in the encoder architectures.

\begin{table*}
    \centering
    \begin{tabular}{|l|c|c|c|l|}
        \hline
        \textbf{Block Type} & \textbf{Number of Layers} & \textbf{Input Channels} & \textbf{Output Channels} & \textbf{Special Functions} \\ \hline
        \textbf{Residual Blocks} & 3 & 7 & 192 & Initial Conv, Residual \\ \hline
        \textbf{Attention Block} & 1 & 192 & 192 & Attention \\ \hline
        \textbf{Residual Blocks} & 3 & 192 & 384 & Residual, Downsampling \\ \hline
        \textbf{Attention Block} & 1 & 384 & 384 & Attention \\ \hline
        \textbf{Residual Blocks} & 3 & 384 & 576 & Residual, Downsampling \\ \hline
        \textbf{Attention Block} & 1 & 576 & 576 & Attention \\ \hline
        \textbf{Residual Blocks} & 3 & 576 & 768 & Residual, Downsampling \\ \hline
        \textbf{Attention Block} & 1 & 768 & 768 & Attention \\ \hline
        \textbf{Residual Blocks} & 2 & 768 & 768 & Residual, Attention \\ \hline
    \end{tabular}
\caption{A comprehensive overview of the layers in the UNet encoder, listed in the order they appear. The architecture starts with the initial convolutional and residual blocks, followed by the attention blocks that enhance the global feature alignment. It continues through subsequent residual and attention blocks, each progressively refining the feature representation by applying downsampling.}
\label{table:unetEnc}
\end{table*}

\begin{table*}
    \centering
    \begin{tabular}{|l|c|c|c|l|}
        \hline
        \textbf{Block Type} & \textbf{Number of Layers} & \textbf{Input Channels} & \textbf{Output Channels} & \textbf{Special Functions} \\ \hline
        \textbf{Residual Blocks} & 2 & 7 & 256 & Initial Conv, Residual \\ \hline
        \textbf{Attention Block} & 1 & 256 & 256 & Attention \\ \hline
        \textbf{Residual Blocks} & 2 & 256 & 512 & Residual, Downsampling \\ \hline
        \textbf{Attention Block} & 1 & 512 & 512 & Attention \\ \hline
        \textbf{Residual Blocks} & 2 & 512 & 768 & Residual, Downsampling \\ \hline
        \textbf{Attention Block} & 1 & 768 & 768 & Attention \\ \hline
        \textbf{Residual Blocks} & 2 & 768 & 1024 & Residual, Downsampling \\ \hline
        \textbf{Attention Block} & 1 & 1024 & 1024 & Attention \\ \hline
        \textbf{Residual Blocks} & 2 & 1024 & 1024 & Residual, Attention \\ \hline
    \end{tabular}
    \caption{Details of the VAE encoder architecture. Similar to the UNet encoder shown in Table \ref{table:unetEnc}, it also uses residual blocks and attention layers to progressively refine the feature representation.}
\label{table:vaeEnc}
\end{table*}

\section{More Qualitative Results}

Figure \ref{fig:qualitative_res_all_appendix} presents the results achieved with the proposed latent diffusion models, PoseNetLdm and PoseNetLdmD. In the second row for each object, the results from the out-of-distribution hand grasps are shown. The results illustrate that employing the HOR-based loss function during training yields superior performance compared to using the identity loss or omitting the pose reconstruction loss altogether. The improvement is particularly evident in the accuracy and fidelity of the reconstructed hand poses, underscoring the effectiveness of the HOR-based loss in enhancing model robustness and generalization to unseen hand configurations.

\begin{figure*}
    \centering
  \includegraphics[width=1.0\textwidth]{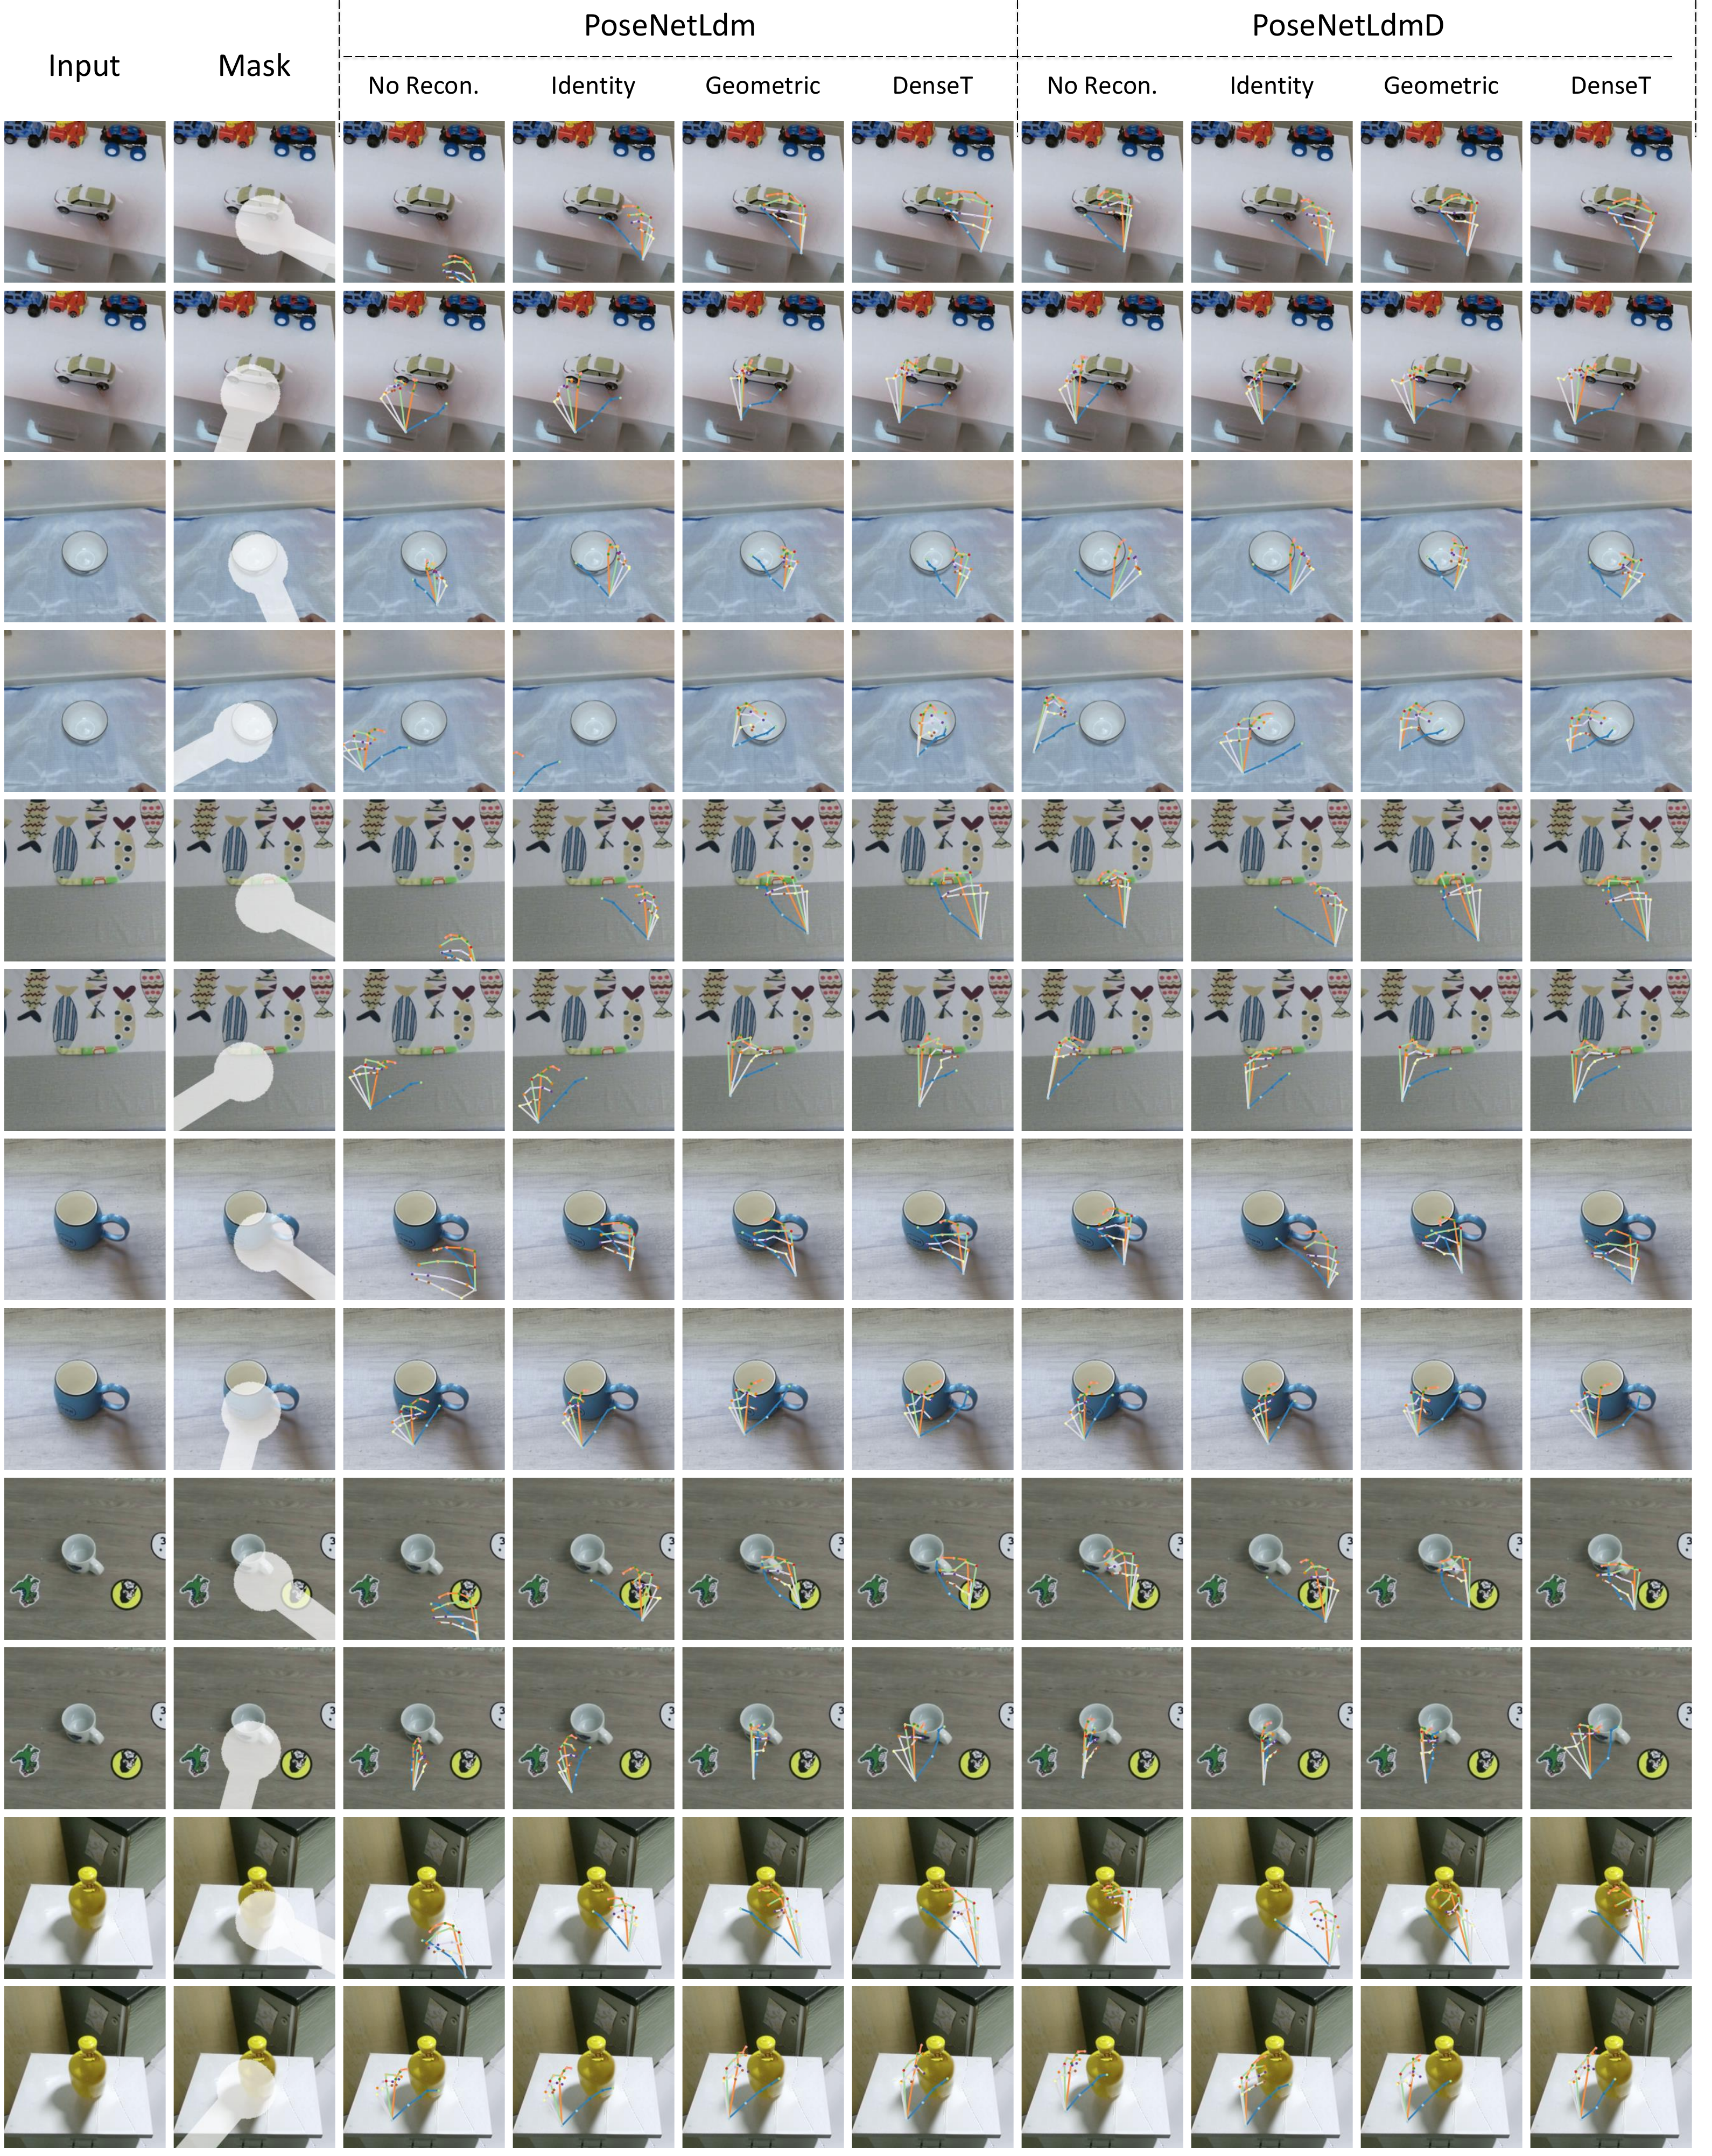}
   \caption{Qualitative comparison of our proposed latent diffusion models for hand pose generation. The first column shows the Input images, and the second column shows the Mask images. The third and fourth columns display the results from the PoseNetLdm and PoseNetLdmD models, respectively. Subsequent columns show the results of our proposed methods under different losses used while training. Each row corresponds to a different test image, demonstrating the performance of each method across a variety of input scenarios. Second row for each object shows the generated hand pose results from out of distribution orientation.}
  \label{fig:qualitative_res_all_appendix}
\end{figure*}
